# Supplementary material for: Rethinking the Alignment of Psychotherapy Dialogue Generation with Motivational Interviewing Strategies
Source: arXiv:2408.06527 source file (2024-12-17)
Supplement: Supplementary file 1 [file appendix-experts.tex]

\clearpage

\begin{appendices}

\section{Assessing statements used in MI expert evaluation}
\label{expert_items}
\end{appendices}

\paragraph{Criteria 1 (EC1):}
The MI strategy effectively guides the generation of the therapist's response. \\
Strongly disagree (1) - Strongly agree (5)
\\
\paragraph{Criteria 2 (EC2):}
The MI strategy does not impact the therapist's response generation. (i.e., the alignment of strategy and the generated therapist’s response are independent). \\
Strongly disagree (1) - Strongly agree (5)
\\
\paragraph{Criteria 3 (EC3):}
The generated therapist's response fits the dialogue context. \\
Strongly disagree (1) - Strongly agree (5)
\\
\paragraph{Criteria 4 (EC4):}
The generated therapist's response aligns with MI principles. \\
Strongly disagree (1) - Strongly agree (5)
\\
\paragraph{Criteria 5 (EC5):}
The quality of the therapist's response is comparable to that of a human therapist. \\
Strongly disagree (1) - Strongly agree (5)
\\
\paragraph{Criteria 6 (EC6):}
The MI strategy aligns with the dialogue context and reflects the MI principles. \\
Strongly disagree (1) - Strongly agree (5)
